# Supplementary material for: Toward verification of the Riemann hypothesis: Application of the Li criterion
Source: arXiv:math-ph/0505052 source file (2005-05-19)
Supplement: Supplementary file 8 [file appendixd.tex]

\centerline{\bf Appendix D:  Tabulated numerical values}
%\begin{table}[h]\centering
\begin{tabular}{|c|c|c|}   
\hline
$k$ & $\lambda_k$ & $\eta_k$ \\
\hline
0 &   $ ~ $     & -0.577216  \\   
1 & 0.0230957   & 0.187546   \\
2 & 0.0923457   & -0.0516886 \\
3 & 0.207639    & 0.0147517 \\
4 & 0.368793    & -0.00452448\\
5 & 0.575543    & 0.0014468 \\
6 & 0.827566    & -0.000471544 \\
7 & 1.12446     & 0.00015518 \\
8 & 1.46576     & -0.0000513452 \\
9 & 1.85092     & 0.0000170414 \\
10 & 2.27934    & $-5.66605 \times 10^{-6}$ \\
11 & 2.75036    & $ 1.88585 \times 10^{-6}$ \\
12 & 3.26326    & $ -6.28055 \times 10^{-7}$ \\ 
13 & 3.81724    & $ 2.09241 \times 10^{-7}$ \\
14 & 4.41148    & $ -6.97247 \times 10^{-8}$ \\
15 & 5.04508    & $ 2.32372 \times 10^{-8}$ \\
16 & 5.71711    & $ -7.74484 \times 10^{-9}$ \\
17 & 6.42658    & $ 2.58144 \times 10^{-9}$ \\
18 & 7.17248    & $ -8.60444 \times 10^{-10}$ \\
19 & 7.95374    & $ 2.86808 \times 10^{-10}$ \\
20 & 8.76928    & $ -9.56012 \times 10^{-11}$ \\
21 & 9.61796    & $ 3.18668 \times 10^{-11}$ \\
22 & 10.4986    & $ -1.06222 \times 10^{-11}$ \\
23 & 11.4101    & $ 3.54072 \times 10^{-12}$ \\
24 & 12.3513    & $ -1.18024 \times 10^{-12}$ \\
25 & 13.3210    & $ 3.93412 \times 10^{-13}$ \\
26 & 14.3179    & $ -1.31137 \times 10^{-13}$ \\
27 & 15.3408    & $ 4.37124 \times 10^{-14}$ \\
28 & 16.3885    & $ -1.45708 \times 10^{-14}$ \\
29 & 17.4599    & $ 4.85694 \times 10^{-15}$ \\
30 & 18.5538    & $ -1.61898 \times 10^{-15}$ \\
\hline
\end{tabular}
%\end{table}

%\begin{table}[h]\centering
\begin{tabular}{|c|c|c|}  
\hline
$k$ & $\lambda_k$ & $\eta_k$ \\
\hline
31 & 19.6689    & $ 5.3966 \times 10^{-16}$ \\
32 & 20.8041    & $ -1.79887 \times 10^{-16}$ \\
33 & 21.9582    & $ 5.99622 \times 10^{-17}$ \\
34 & 23.1301    & $ -1.99874 \times 10^{-17}$ \\
35 & 24.3188    & $ 6.66247 \times 10^{-18}$ \\
36 & 25.5232    & $ -2.22082 \times 10^{-18}$ \\
37 & 26.7422    & $ 7.40274 \times 10^{-19}$ \\
38 & 27.9749    & $ -2.46755 \times 10^{-19}$ \\
39 & 29.2202    & $ 8.22527 \times 10^{-20}$ \\
40 & 30.4774    & $ -2.74176 \times 10^{-20}$ \\
41 & 31.7454    & $ 9.13919 \times 10^{-21}$ \\
42 & 33.0236    & $ -3.0464 \times 10^{-21}$ \\
43 & 34.3111    & $ 1.01547 \times 10^{-21}$ \\
44 & 35.6072    & $ -3.38488 \times 10^{-22}$ \\
45 & 36.9113    & $ 1.12829 \times 10^{-22}$ \\
46 & 38.2227    & $-3.76098 \times 10^{-23}$ \\
47 & 39.5408    & $ 1.25366 \times 10^{-23}$ \\
48 & 40.8653    & $ -4.17887 \times 10^{-24}$ \\
49 & 42.1955    & $ 1.39295 \times 10^{-24}$ \\
50 & 43.5311    & $ -4.64318 \times 10^{-25}$ \\
51 & 44.8718    & $ 1.54773 \times 10^{-25}$ \\
52 & 46.2172    & $ -5.15909 \times 10^{-26}$ \\
53 & 47.5671    & $ 1.71970 \times 10^{-26}$ \\
54 & 48.9214    & $ -5.73232 \times 10^{-27}$ \\
55 & 50.2798    & $ 1.91077 \times 10^{-27}$ \\
56 & 51.6423    & $ -6.36925 \times 10^{-28}$ \\
57 & 53.0089    & $ 2.12308 \times 10^{-28}$ \\
58 & 54.3795    & $ -7.07695 \times 10^{-29}$ \\
59 & 55.7542    & $ 2.35898 \times 10^{-29}$ \\
60 & 57.1331    & $ -7.86327 \times 10^{-30}$ \\
\hline
\end{tabular}

\begin{tabular}{|c|c|c|}  
\hline
$k$ & $\lambda_k$ & $\eta_k$ \\
\hline
61 & 58.5163    & $ 2.62109 \times 10^{-30}$ \\
62 & 59.9039    & $ -8.73697 \times 10^{-31}$ \\
63 & 61.2962    & $ 2.91232 \times 10^{-31}$ \\
64 & 62.6934    & $ -9.70775 \times 10^{-32}$ \\
65 & 64.0957    & $ 3.23591  \times 10^{-32}$ \\ 
66 & 65.5033    & $ -1.07864 \times 10^{-32}$ \\
67 & 66.9167    & $  3.59546 \times 10^{-33}$ \\
68 & 68.3361    & $ -1.19849 \times 10^{-33}$ \\
69 & 69.7618    & $  3.99496 \times 10^{-34}$ \\
70 & 71.1942    & $ -1.33165 \times 10^{-34}$ \\
71 & 72.6337    & $ 4.43884 \times 10^{-35}$ \\
72 & 74.0805    & $ -1.47961 \times 10^{-35}$ \\
73 & 75.5350    & $ 4.93205 \times 10^{-36}$ \\
74 & 76.9976    & $ -1.64402 \times 10^{-36}$ \\
75 & 78.4686    & $ 5.48005 \times 10^{-37}$ \\
76 & 79.9484    & $ -1.82668 \times 10^{-37}$ \\
77 & 81.4373    & $ 6.08895 \times 10^{-38}$ \\
78 & 82.9357    & $ -2.02964 \times 10^{-38}$ \\
79 & 84.4437    & $ 6.76550 \times 10^{-39}$ \\
80 & 85.9617    & $ -2.25516 \times 10^{-39}$ \\
81 & 87.4900    & $ 7.51722 \times 10^{-40}$ \\
82 & 89.0288    & $ -2.50574 \times 10^{-40}$ \\
83 & 90.5782    & $ 8.35246 \times 10^{-41}$ \\
84 & 92.1386    & $ -2.78415 \times 10^{-41}$ \\
85 & 93.7099    & $ 9.28051 \times 10^{-42}$ \\
86 & 95.2924    & $ -3.09350 \times 10^{-42}$ \\
87 & 96.8862    & $ 1.03117 \times 10^{-42}$ \\
88 & 98.4912    & $ -3.43723 \times 10^{-43}$ \\
89 & 100.1076   & $ 1.14574 \times 10^{-43}$ \\
90 & 101.7352   & $ -3.81914 \times 10^{-44}$ \\
\hline
\end{tabular}

\begin{tabular}{|c|c|c|}  
\hline
$k$ & $\lambda_k$ & $\eta_k$ \\
\hline
91 & 103.3741   & $ 1.27304 \times 10^{-44}$ \\
92 & 105.0242   & $ -4.24349 \times 10^{-45}$ \\
93 & 106.6852   & $ 1.41450 \times 10^{-45}$ \\
94 & 108.3572   & $ -4.71500 \times 10^{-46}$ \\
95 & 110.0398   & $ 1.57166 \times 10^{-46}$ \\
96 & 111.7328   & $ -5.23888 \times 10^{-47}$ \\
97 & 113.4361   & $ 1.74629 \times 10^{-47}$ \\
98 & 115.1492   & $ -5.82098 \times 10^{-48}$ \\
99 & 116.8719   & $ 1.94032 \times 10^{-48}$ \\
100 & 118.6038  & $ -6.46775 \times 10^{-49}$ \\
\hline
\end{tabular}
%\end{table}
